# Supplementary material for: Temperature and thickness dependence of the thermal conductivity in 2D ferromagnet Fe$_3$GeTe$_2$
Source: arXiv:2307.12863 source file (2023-07-24)
Supplement: Supplementary file 1 [file Supp.pdf]

## *Supplementary information of*

# Temperature and thickness dependence of the thermal conductivity in 2D ferromagnet $Fe_3GeTe_2$

M. S. Claro,[1] J. Corral-Sertal,[1] A. Otero-Fumega,[2] S. Blanco-Canosa,[3, 4] M. Súarez-Rodríguez,[5] L. Hueso,[5, 4]
V. Pardo,[6, 7] and F. Rivadulla[1]

[1)]CiQUS, Centro Singular de Investigacion en Quimica Bioloxica e Materiais Moleculares, Departamento de Quimica-Fisica, Universidade de Santiago de Compostela, 15782-Santiago de Compostela,
Spain.

[2)]Department of Applied Physics, Aalto University, FI-00076 Aalto, Finland

[3)]Donostia International Physics Center (DIPC), 20018 San Sebastían, Spain

[4)]IKERBASQUE, Basque Foundation for Science, 48013 Bilbao, Spain

[5)]CIC nanoGUNE BRTA, Donostia-San Sebastían, Spain

[6)]Departamento de Física Aplicada, Universidade de Santiago de Compostela, E-15782 Santiago de Compostela,
Spain

[7)]Instituto de Materiais iMATUS, Universidade de Santiago de Compostela, E-15782 Campus Sur s/n, Santiago de Compostela, Spain

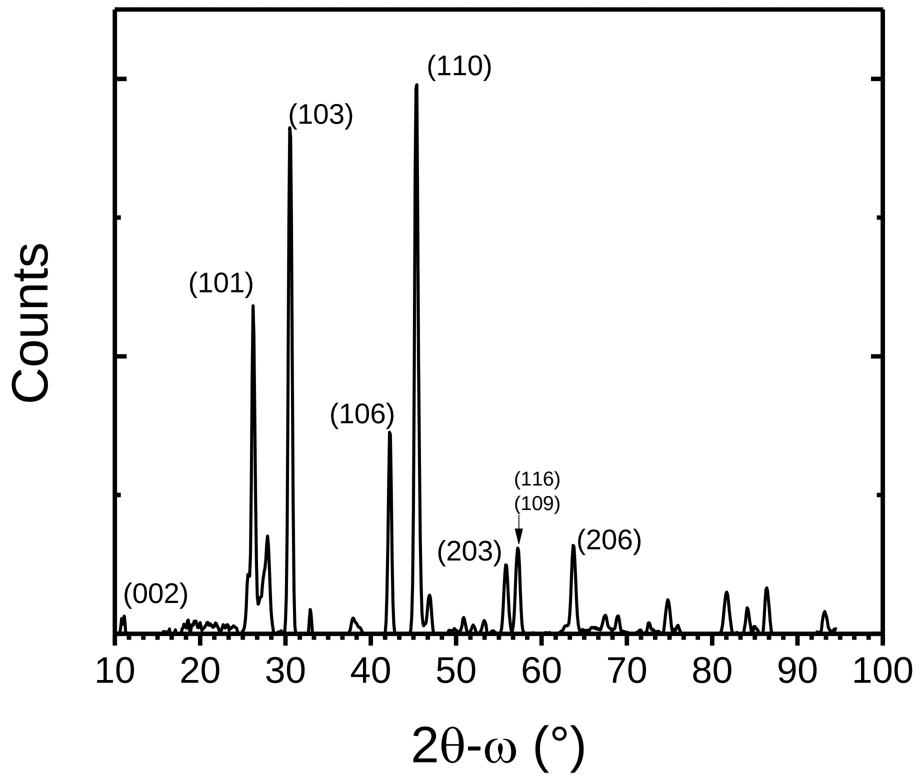


Figure S1. X-ray powder diffraction pattern with main crystallographic planes identified from the $Fe_3GeTe_2$ crystals used.

We define the sensitivity of the fitting parameter α as the logarithmic derivative of the FDTR phase-shift (ϕ) with respect to the parameter. If that parameter is set as α, then:

$$S_\alpha = \frac{d\ \varphi}{d\ ln\alpha}$$

The sensitivity for the parameters of interest (k, G1 and G2) is higher between 1 MHz to 50 MHz, the range used in the fittings.

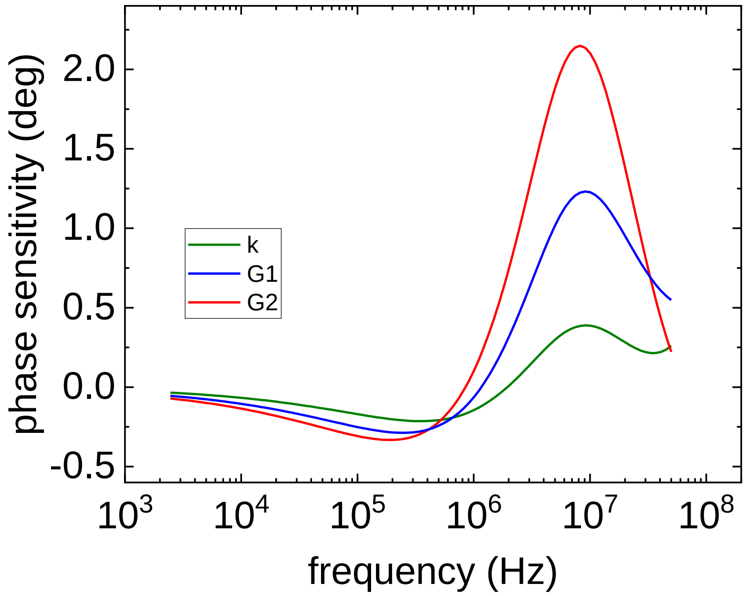


Figure S2. Phase sensitivity of out-of-plane thermal conductivity of $Fe_3GeTe_2$ (k), G1 and G2 TBCs in the Frequency Domain Thermoreflectance (FDTR) experiment.

Due to the strong correlation between the G1 and G2 parameters, in practice, only the sum G1+G2 is considered in the fitting. Figure S3 shows the variation of this parameter with temperature. These values were applied in the fitting presented in Figure 5a.

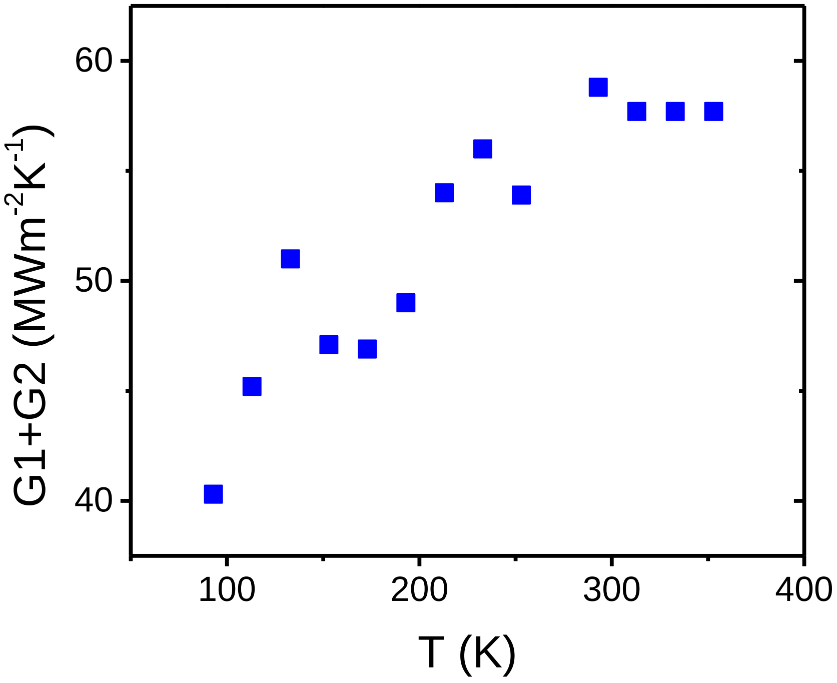


Figure S3. Total thermal boundary conductivity (TBC) G1+G2 TBCs extracted from the FTDR phase-shift fittings.

To apply an external magnetic field to the thin films, we have used permanent magnets made of NdFeB (N45). These magnets can be placed and removed keeping the measured spot fixed.

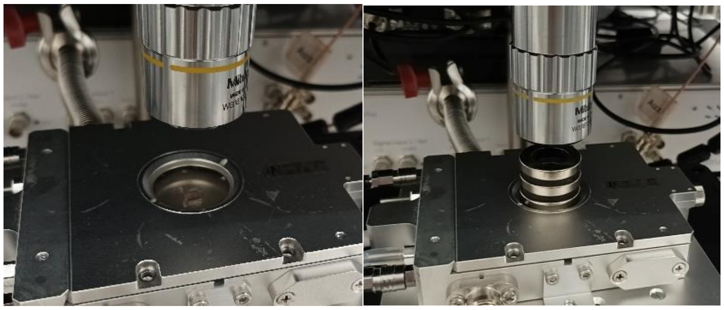

Figure S4. Sample inside the optical cryostat below the FDTR confocal lenses (left) and added toroidal magnets for measurements with a magnetic field (right).

The toroidal shape allows the transmission of the pump and probe laser without any interference. Moreover, this shape creates a considerably uniform and constant out-of-plane magnetic field. Since

magnetization and geometry are well known, the field was determined using Finite Element Method (FEMM 4.2) (Figure S5) from which we estimate a field of 56 mT in the sample plane.

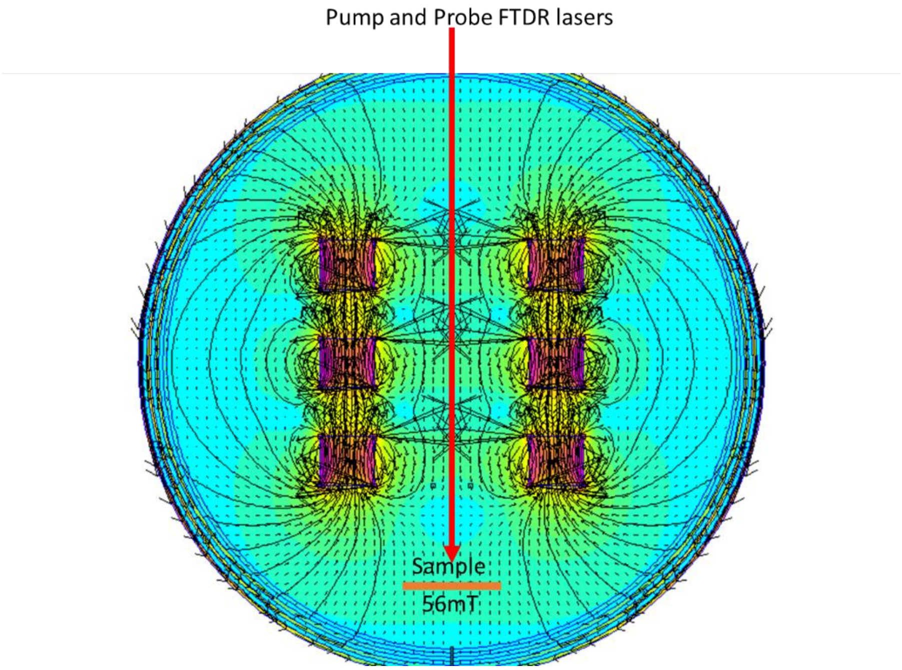


Figure S5. Finite-Element (FEM) simulation of the Magnetic Field applied to the sample during the FDTR experiment with toroidal permanent magnets.
